# Supplementary material for: AutoDenoise: Automatic Data Instance Denoising for Recommendations
Source: arXiv:2303.06611 source file (2023-03-12)
Supplement: Supplementary file 1 [file 6Appendix.tex]

\section{Datasets}
\label{sec:dataset}
We evaluate the model performance of IDPN and baselines on three public datasets with different densities, \textbf{MovieLens1M\footnote{\url{https://grouplens.org/datasets/movielens/1m/}}}, \textbf{KuaiRec-Small\footnote{\url{https://github.com/chongminggao/KuaiRec}}}, and \textbf{Netflix\footnote{\url{https://www.kaggle.com/datasets/netflix-inc/netflix-prize-data}}}, 
\begin{itemize}[leftmargin=*]
    \item \textbf{MovieLens1M
    % \footnote{\url{https://grouplens.org/datasets/movielens/1m/}}
    :} This is a widely-used benchmark dataset for click-through rate prediction, which is collected by GroupLens Research from MovieLens website. 
    We regard ratings higher than $3$ as `click', otherwise `unclick'. 
    This dataset contains $1,000,000$ interaction logs of $6,040$ users on $3,706$ items, implying a moderate density $10e^6/(6040 \times 3706)= 4.47\%$.
    
    \item \textbf{KuaiRec-Small
    % \footnote{\url{https://github.com/chongminggao/KuaiRec}}
    :} KuaiRec~\cite{gao2022kuairec} is a real-world user-video interaction dataset from a popular online video platform, Kuaishou. 
    KuaiRec-Small is a small version of KuaiRec, which contains all users' feedback on all videos. There are $1,411$ users and $3,327$ videos in this dataset. The number of user-video interactions is 4,676,570. Thus, KuaiRec-Small has a very high density that $4676570/(1411 \times 3327)=99.62\%$.
    
    \item \textbf{Netflix
    % \footnote{\url{https://www.kaggle.com/datasets/netflix-inc/netflix-prize-data}}
    :} This dataset contains over $100$ million ratings from $480,000$ Netflix customers over $17,000$ movies. 
    Similar to MovieLens1M, ratings higher than $3$ are regarded as `click'. 
    We randomly sample $1$ million interactions from the whole dataset to conduct faster experiments. In our dataset, there are 290,078 users and $16,209$ items with 1 million interaction logs, where the density is $10e^6/(290,078 \times 16,209)=0.02\%$.
\end{itemize}

For all datasets, we randomly select $80\%$ as the training set, $10\%$ as the validation set, and the remaining $10\%$ as the test set.  

Please note that we split all data as `click' or `unclick' and regard them as noisy data, which is different from previous denoising works~\cite{wang2021denoising,wang2021implicit,wang2022learning}. They regard all data as `click', where noises are those 'click' behaviors with less than $3$ scores (false positive).

\section{Implementation Details}
\label{sec:implemantation}
% The implementation of \name 
% can be divided into the model structure design and the training algorithm design. 

% \subsection{Model Structure Design}
The model structure of \name mainly consists of the policy network and the RS model. We implement the policy network and adapt the RS model from the public recommender system library\footnote{https://github.com/rixwew/pytorch-fm}. 

(a) \textit{Policy Network}: it totally consists of the embedding layer, MLP layer, and output layer. We set the embedding size in the embedding layer and the dimension size of all fully-connected layers in MLP as $d=16$. To generate probabilities for every instance, we set the dimension of the output layer as 2. Specifically, when a $F$ feature fields instance, it will first be transformed into a $F \times d$ matrix. And then, the transformed matrix will be flattened into a vector with dimension $F*d$ and go through two fully-connected MLP layers without dimensional change, where every mlp layer consists of a linear layer, a batch normalization operation, a ReLU activation function, and dropout(\textit{rate = 0.2}). Finally, the output from the MLP layer will be transformed into a 2-dimension probability with \textit{softmax} activation, which is the output of the policy network.

(b) \textit{RS Model}: every RS model in this library is implemented individually, for fair comparison as in Section~\ref{sec:overall_performance}, we consider the same parameter settings for our tested ones. Specifically, the embedding size and the dimension size for all intermediate layers are all set to 16, and the output layer, which in the binary classification setting, uses \textit{sigmoid} activation.

% \subsection{Training Algorithm Design}
% For the training algorithm design, we follow the reinforcement learning algorithm.

\section{Hyper-Parameter Tuning}
\label{sec:hyper_param}
For our proposed framework, \name, we have tried some combinations of the hyper-parameters for better performance through several experiments. The results are shown in Table~\ref{table:hyper}, where  ``Best choice'' in the last column represents the optimal settings. 
% Specifically, for the  ``Selection ratio'' hyper-parameter, which is tested from 80\% to 99\%, the best ones for Movielen1M, KuaiRec-Small and Netflix are 98\%, 97\% and 95\%, respectively. For ``Warm-up epoch'', which was tuned from 2 to 6, performs the best with 4 epochs in Movielen1M, while 3 epochs in the others.

\begin{table}[!t]
\small
\caption{Hyper-parameters tuning for \name}
\label{table:hyper}
\begin{tabular}{@{}cccc@{}}
\toprule
Dataset                        & Hyper-parameter                      & Tuning range                 & Best choice           \\ \midrule
\multirow{2}{*}{Movielen1M}    & Selection ratio                      & 80-99\%                      & 98\%                 \\\cmidrule(l){2-4} 
                               & Warm-up epoch                        & 2-6                          & 4                    \\ \midrule
\multirow{2}{*}{KuaiRec-Small} & Selection ratio                      & 80-99\%                      & 97\%                 \\\cmidrule(l){2-4} 
                               & Warm-up epoch                        & 2-6                          & 3                    \\ \midrule
\multirow{2}{*}{Netflix}       & Selection ratio                      & 80-99\%                      & 95\%                 \\\cmidrule(l){2-4} 
                               & Warm-up epoch                        & 2-6                          & 3                    \\ \midrule
\multirow{4}{*}{All Dataset}   & \makecell{Selection method \\in Searching phase}  & \makecell{Individual / \\Top-k selection} & \makecell{Individual \\selection} \\\cmidrule(l){2-4} 
                               & \makecell{Selection method \\in Validation phase}  & \makecell{ Individual / \\Top-k selection} & \makecell{ Top-k\\ selection}      \\ \bottomrule
\end{tabular}
\vspace{-3mm}
\end{table}

\section{Baselines}
\label{sec:baseline}
We briefly introduce baselines in this section, including instance selection methods (Drop3~\cite{wilson2000reduction}, BDIS~\cite{Chen_Cao_Xing_Liang_2022}, LSBo~\cite{leyva2015three}, LSSm~\cite{leyva2015three}) and instance denoising methods (T\_CE~\cite{wang2021denoising}, R\_CE~\cite{wang2021denoising}):
\begin{itemize}[leftmargin=*]
    \item \textbf{Drop3~\cite{wilson2000reduction}:} It is one of the models proposed by \citet{wilson2000reduction}, which removes instances in two steps and obtains the selection result. The first stop of Drop3 is the noise filter. In this step, Drop3 removes all samples misclassified by KNN. Then, the remaining instances are sorted by their distances to the decision boundary, where instances far from the boundary would be dropped. 
    \item \textbf{BDIS~\cite{Chen_Cao_Xing_Liang_2022}:} In this paper, \citet{Chen_Cao_Xing_Liang_2022} propose an instance selection framework for large-scale data with a solid foundation of bayesian decision theory. They first illustrate the theoretical support of previous KNN-based instance selection methods. Then, based on their theory, three kinds of relationships are established between reducible, irreducible, and deleterious instances to construct local homogeneous clusters for selection.
    \item \textbf{LSBo, LSSm~\cite{leyva2015three}:} Different from previous distance-based solutions for instance selection, these two methods are constructed based on the local set consumption.
    \item \textbf{T\_CE, R\_CE~\cite{wang2021denoising}:} Both methods are from ADT~\cite{wang2021denoising}, which adaptively learns to detect false positive user-item interactions for a more robust recommendation. The main idea of ADT is that false positive interactions always tend to obtain a larger loss value during the model training. ADT designs T\_CE to truncate large losses, or R\_CE to assign low weight to noises, which could be  regarded as selection-based and reweighting-based denoising methods, respectively.
\end{itemize}
